# Supplementary material for: How Transformers Get Rich: Approximation and Dynamics Analysis
Source: arXiv:2410.11474 source file (2025-01-29)
Supplement: Supplementary file 1 [file proof_dynamics.tex]

\vspace{1.cm}

\section{Proofs in Section \ref{section: optimization}}

\subsection{Stage II}

% \begin{figure}
%     \centering
%     \includegraphics[width=0.99\linewidth]{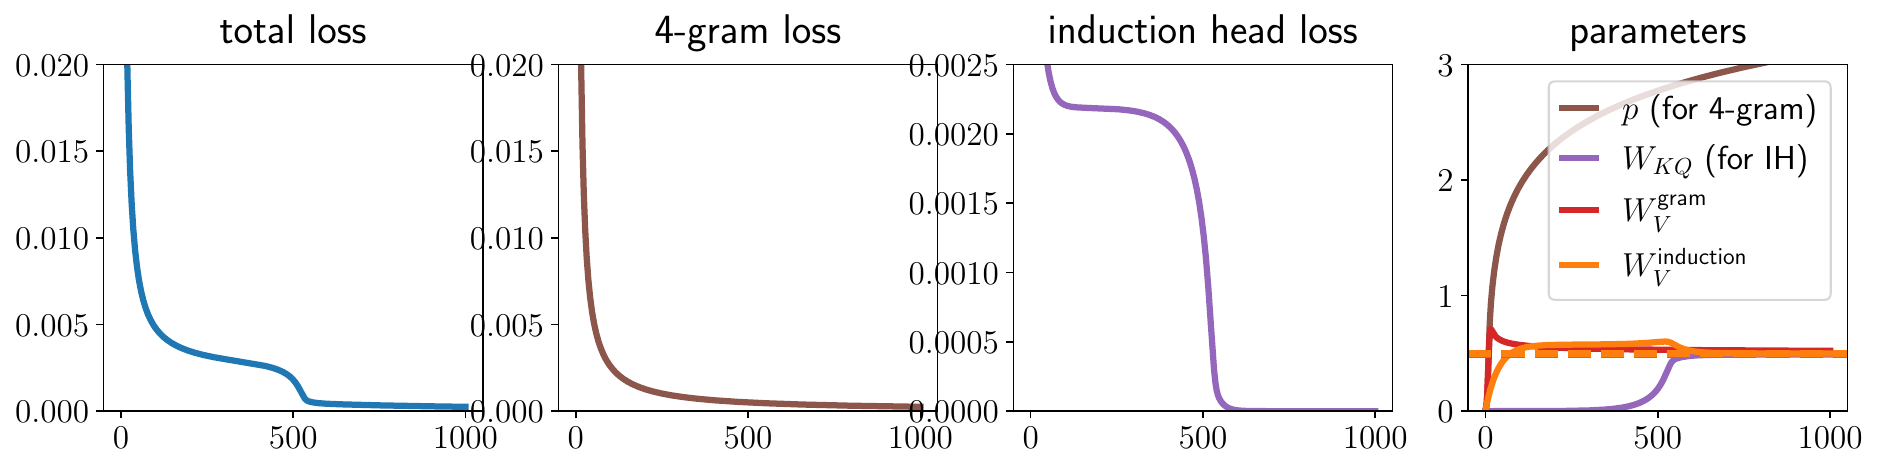}
%     \caption{Phase change, $\alpha=10$}
%     \label{fig: phase change}
% \end{figure}

$$f^*(x) = \frac{1}{1+\alpha}\left( \alpha x_{L-2} + \frac{1}{L-2}\sum_{s=2}^{L-1} \exp (w^* x_L x_{s-1})x_s\right)$$

$$f_{w.p}(x) = \frac{1}{1+\alpha}\left( \alpha\sum_{s=2}^{L-1}\sm(-p(L-1-s))x_{s-1}+\frac{1}{L-2}\sum_{s=2}^{L-1}\exp(w x_L x_{s-1})x_s \right)$$

\begin{align*}
    \mathcal{L}(w,p) & = \frac{1}{2(1+\alpha)^2}\mathop{\bbE}\limits_{\bX\sim\bbN(0,1)^L}\Bigg[\alpha x_{L-2}-\alpha\sum_{s=2}^{L-1}\sm(-p(L-1-s))x_{s-1}
    \\& \quad\quad\quad\quad\quad\quad\quad\quad\quad\quad +\frac{1}{L-2}\sum_{s=2}^{L-1}\exp(w^*x_L x_{s-1})x_s - \frac{1}{L-2}\sum_{s=2}^{L-1}\exp(w x_L x_{s-1})x_s \Bigg]
    \\& = \frac{1}{2(1+\alpha)^2}\mathop{\bbE}\limits_{\bX\sim\bbN(0,1)^L}\Bigg[ \alpha^2 x_{L-2}^2 + \alpha^2\sum_{s=2}^{L-1}\sm^2(-p(L-1-s)) x_{s-1}^2
    \\& \quad\quad\quad\quad\quad\quad\quad\quad\quad\quad + \left( \frac{1}{L-2} \right)^2 \sum_{s=2}^{L-1}\exp(2w^*x_Lx_{s-1})x_s^2 + \left( \frac{1}{L-2} \right)^2 \sum_{s=2}^{L-1}\exp(2wx_Lx_{s-1})x_s^2
    \\& \quad\quad\quad\quad\quad\quad\quad\quad\quad\quad -2\alpha^2\sm(0)x_{L-2}^2
    \\& \quad\quad\quad\quad\quad\quad\quad\quad\quad\quad + \frac{2\alpha}{L-2}\exp(w^* x_L x_{L-3})x_{L-2}^2 - \frac{2\alpha}{L-2}\exp(w x_L x_{L-3})x_{L-2}^2
    \\& \quad\quad\quad\quad\quad\quad\quad\quad\quad\quad - \frac{2\alpha}{L-2}\sum_{s=2}^{L-2}\sm(-p(L-2-s))\exp(w^* x_L x_{s-1})x_s^2
    \\& \quad\quad\quad\quad\quad\quad\quad\quad\quad\quad + \frac{2\alpha}{L-2}\sum_{s=2}^{L-2}\sm(-p(L-2-s))\exp(w x_L x_{s-1})x_s^2
    \\& \quad\quad\quad\quad\quad\quad\quad\quad\quad\quad - \frac{2}{(L-2)^2}\sum_{s=2}^{L-1}\exp((w+w^*)x_L x_{s-1})x_s^2
\end{align*}

\begin{lemma}
    $\mathop{\bbE}\limits_{X,Y,Z}\exp(aXY)\bZ^2 = (1-a^2)^{-1/2}$, $a<1$.
\end{lemma}
\begin{proof}
    \begin{align*}
        &\quad \int\exp(aXY)Z^2\left(\frac{1}{2\pi}\right)^{-3/2}\exp(-\frac{1}{2}X^2-\frac{1}{2}Y^2-\frac{1}{2}Z^2)\ dX dY dZ
        \\ & = \int\frac{1}{2\pi}\exp(-\frac{1}{2}(X-aY)^2-\frac{1}{2}Y^2+\frac{1}{2}a^2Y^2)\ d(X-aY)dY
        \\ & = \int\frac{1}{\sqrt{2\pi}}\exp(-\frac{1}{2}W^2)\ dW \ (W = (1-a^2)^{1/2}Y )
        \\ & = (1-a^2)^{-1/2}
    \end{align*}
\end{proof}

\begin{align*}
    \mathcal{L} & = \frac{1}{2(1+\alpha)^2} \Bigg[ \alpha^2 + \frac{1}{L-2}(1-4w^{*2})^{-1/2} + \frac{2\alpha}{L-2}\sm(-p(L-3))(1-w^{*2})^{-1/2}
    \\ & \quad\quad\quad\quad\quad\quad -\frac{2}{L-2}(1-(w+w^*)^2)^{-1/2} + \frac{1}{L-2}(1-4w^2)^{-1/2}
    \\ & \quad\quad\quad\quad\quad\quad -\frac{2\alpha}{L-2}\sm(-p(L-3))(1-w^2)^{-1/2}
    \\ & \quad\quad\quad\quad\quad\quad +\alpha^2\sum_{s=2}^{L-1}\sm^2(-p(L-1-s)) - 2\alpha^2\frac{1}{M(p)} \Bigg],
\end{align*}
 where $M(P) = \sum_{s=2}^{L-1}\exp(-p(L-1-s)) = \sum_{s=0}^{L-3}\exp{-ps} = \frac{1-e^{-p(L-2)}}{1-e^{-p}}$.

\begin{align*}
    \frac{dw}{dt} & = \frac{1}{2(1+\alpha)^2}\Bigg[\frac{2}{L-2}(1+(w+w^*)^2)^{-3/2}(w+w^*)
    \\ &\quad\quad\quad\quad\quad -\frac{2}{L-2}(1-4w^2)^{-3/2}(2w)
    \\ &\quad\quad\quad\quad\quad +\frac{2\alpha}{L-2}\sm(-p(L-3))(1-w^2)^{-3/2}w \Bigg]
\end{align*}

\begin{align*}
    \frac{dp}{dt} & = \frac{\alpha}{(1+\alpha)^2}\frac{m(p)}{M(p)^2}\Bigg[\alpha\left(\frac{m(2p)}{m(p)}-\frac{M(2p)}{M(p)}+1\right)
    \\ & \quad\quad\quad\quad+\frac{1}{L-2}\Big((L-3)\exp(-p(L-3))-\exp(-p(L-3))\Big)\cdot\left((1-w^{*2})^{-1/2}-(1-w^2)^{-1/2}\right)
    \Bigg],
\end{align*}
where $m(p) = \sum_{s=1}^{l-3}s\exp(-ps) = \frac{e^{-p}-(L-2)e^{-p(L-2)}+(L-3)e^{-p(L-1)}}{(1-e^{-p})^2}$.

\begin{lemma}
    $\frac{M(2p)}{M(p)}\leq 1$.
\end{lemma}
\begin{proof}
    $$\frac{M(2p)}{M(p)} = \frac{1+e^{-p(L-2)}}{1+e^{-p}}$$
    \begin{align*}
        \left(\frac{M(2p)}{M(p)}\right)' & = \frac{-(L-2)-(L-3)e^{-p}+e^{-p(L-1)}}{(1+e^{-p})^2}
        \\ & \leq \frac{-(L-2)-(L-4)e^{-p}}{(1+e^{-p})^2}
        \\ & \leq 0.
    \end{align*}
\end{proof}

$$\frac{dp}{dt}\leq\frac{\alpha}{(1+\alpha)^2}\frac{m(p)}{M(p)^2}\Bigg[\ \alpha\frac{m(2p)}{m(p)}-\frac{1}{L-1}\left(\frac{1}{1-w^{*2}}\right)^{1/2} \Bigg]$$

\begin{lemma}
    $\int_A^B\frac{M(p)^2}{m(p)}\ dp\sim e^B-e^A$.
\end{lemma}
\begin{proof}
    \begin{align*}
        I & := \int_A^B\frac{\left(\sum_{s=0}^{L-3}\exp(-ps)\right)^2}{\sum_{s=1}^{L-3}s\exp(-ps)}\ dp
        \\ & = \int_{e^{-B}}^{e^{-A}}\frac{\left(\sum_{s=0}^{L-3}m^s\right)^2}{\sum_{s=1}^{L-3}sm^s}\cdot\frac{1}{m}\ dm\ (m = e^{-p})
        \\ & = \int_{e^{-B}}^{e^{-A}}\frac{(1-m^{L-2})^2}{m^2(1-(L-2)m^{L-3}+(L-3)m^{L-2})}\ dm
        \\ & = \int_{e^{-B}}^{e^{-A}}\frac{1}{m^2}+m^{L-5}\cdot\frac{(L-2)-(L-1)m+m^{L-1}}{1-(L-2)m^{L-3}+(L-3)m^{L-2}}\ dm
    \end{align*}
    $$\frac{d}{dm}(L-2)-(L-1)m+m^{L-1} = (L-1)(m^{L-2}-1)\leq 0$$
    $$\frac{d}{dm}1-(L-2)m^{L-3}+(L-3)m^{L-2} = (L-2)(L-3)(m^{L-3}-m^{L-4})\geq 0$$
    $$\frac{(L-2)-(L-1)m+m^{L-1}}{1-(L-2)m^{L-3}+(L-3)m^{L-2}}\leq L-2$$
    \begin{align*}
        I & \leq \int_{e^{-B}}^{e^{-A}}\frac{1}{m^2}+m^{L-5}(L-2)
        \\ & = e^B-e^A+\frac{L-2}{L-4}\left(e^{-A(L-4)}-e^{-B(L-4)}\right)
    \end{align*}
\end{proof}

\begin{lemma}
    $\frac{m(2p)}{m(p)}$ is decreasing.
\end{lemma}
\begin{proof}
    $t:=e^{-p}$, numerator of $-\left(\frac{m(2p)}{m(p)}\right)'$ is 
    \begin{align*}
        & \sum_{s=1}^{L-3}2s^2 t^{2s}\sum_{s=1}^{L-3}st^s-\sum_{s=1}^{L-3}st^{2s}\sum_{s=1}^{L-3}s^2 t^s
        \\ & \sum_{i,j = 1}^{L-3}(2i-j)ijt^{2i+j}
        \\ & \sum_{k=3}^{3L-9}t^k\sum_{k = 2i+j}ij(2i-j)
        \\ & \sum_{k=3}^{3L-9}\frac{1}{2}t^k\sum_{i}2i(k-2i)(4i-k)
    \end{align*}
    For even terms
    $$\sum_{i=1}^{L-3}i(2l-2i)(4i-2l) = 4\sum_{i=1}^{L-3}i(l-1)(2i-l) = 0$$
    For odd terms
    $$\sum_{i=1}^{L-3}i(2l+1-2i)(4i-2l-1) = \sum_{i=1}^{L-3}i(-8i^2+(2l+6)i-(2l+1)^2) = \frac{(L-3)(L-2)}{2}$$
    Hence $\left(\frac{m(2p)}{m(p)}\right)'<0$.
\end{proof}

Set $g(x) = x(1-x^2)^{-3/2}$, since
$$g'(x) = (1-x^2)^{-3/2}\frac{2x^2+1}{1-x^2}$$
$$g''(x) = (1-x^2)^{-7/2}\left[5x(2x^2+1)+4x(1-x^2)\right]\geq 0$$
$g$ is an increasing convex function on $(0,1)$.

\begin{align*}
    (1+\alpha)^2(L-2)\frac{dw}{dt} & = g(w+w^*)-g(2s)
    \\ & \geq g'(2w)(w^*-w)
    \\ & \geq w^*-w
\end{align*}

\paragraph{Phase I.} w increases from $0$ to $0.01w^*$ on $[0,T_I]$.
$$\frac{dw}{dt} \approx \frac{1}{(1+\alpha)^2(L-2)}\left[ 1-(w+w^*)^2 \right]^{-3/2}(w+w^*) $$
\begin{align*}
    T_I & \approx (1+\alpha)^2(L-2)\int_{w^*}^{0.01w^*}\frac{(1-w^2)^{-3/2}}{w}\ dw
    \\ & := (1+\alpha)^2(L-2)C(w^*)
\end{align*}
By the mean value theorem for integrals $C(w^*)\approx 0.0064952$.

\paragraph{Phase II.} w increases from $0.01w^*$ to $\frac{w^*}{1+\beta}$ on $[T_I,T_{II}]$.
$$w\leq 0.01w^*\exp(\frac{\beta t}{(1+\alpha)^2(L-2)})$$
$$T_{II}-T_I\leq\frac{(1+\alpha)^2(L-2)}{\beta}\ln\left( \frac{1}{0.01(1+\beta)} \right)$$

We assume $L\sim 10^Q$ for sufficiently large $Q$. As for $p$, we prove that $p$ reaches a sufficiently large $p_I$ in phase I and keeps non-decreasing and smaller than $p_{II}$ until the end of phase II. 

Notice that the sufficient and necessary condition for sufficiently large $p$ to be no-decreasing is 
$$C(p) = \frac{m(2p)}{m(p)}\sim e^{-p}\geq \frac{2}{\alpha(L-2)}(1-w^{*2})^{-1/2},$$
We take 
$$p_I = \frac{1}{2}\ln L+ \ln\left( \frac{\alpha(1-w^{*2})^{1/2}}{2} \right)$$
$$p_{II} = \ln L+ \ln\left( \frac{\alpha(1-w^{*2})^{1/2}}{2} \right)$$
and construct a lower solution of $p$ denoted as $q$
$$\frac{dq}{dt}=\begin{cases} \frac{\alpha^2}{2(1+\alpha)^2}\frac{m(q)}{M(q)^2}C(p_I),&\  0\leq q\leq t_I \\ \frac{\alpha^2}{2(1+\alpha)^2}\frac{m(q)}{M(q)^2}C(p_{II}),\ & t_{I}\leq q\leq t_{II}.
\end{cases}$$
where $t_I$ is the time $q$ reaches $p_I$, $t_{II}$ is the time $q$ reaches $p_{II}$,

The time cost for $q$ increasing from $A$ to $B$ is 
$$(e^B-e^B)\left( \frac{\alpha^2}{2(1+\alpha)^2}C(B) \right)^{-1},$$
where $C(B):=\frac{m(2B)}{m(B)}$.

Starting from A, if q continues to increase over time t and remains less than B during this period, then q can reach:
$$\ln\left( \frac{\alpha^2}{2(1+\alpha)^2}C(B)t+e^A \right).$$

By calculation, we obtain that $t_I\leq T_I$ and 
$$t_{II}\sim\frac{(1+\alpha)^2(1-w^{*2})}{2}(L-2)^2$$
$$T_{II}\sim C(w^*)(1+\alpha)^2(L+2)+\frac{(1+\alpha)^2(L-2)}{\beta}\ln\left( \frac{1}{0.01(1+\beta)} \right)$$
hence $t_{II}>T_{II}$.

\subsection{Stage I}

$$y_s = \sum_{\tau=1}^{s-1}\sm_s(-\tilde{p}(s-1-\tau))x_{\tau}$$

$$f^* = \alpha x_{L-2} + \frac{1}{L-2}\sum_{s=2}^{L-1}\exp(w^* x_L x_{s-1})x_s$$

\begin{align*}
f_{\theta} & = \alpha\sum_{s=2}^{L-1}\sm(-p(L-1-s))\cdot\left(\sum_{\tau=1}^{s-1}\sm_s(-\tilde{p}(s-1-\tau))x_{\tau}\right)+\frac{1}{L-2}\sum_{s=2}^{L-1}x_s
\\& = \frac{\alpha}{L-2}\sum_{\tau=1}^{L-2}\left(\sum_{s = \tau+1}^{L-1}\sm_s(-\tilde{p}(s-1-\tau))\right)x_{\tau}+\frac{1}{L-2}\sum_{s=2}^{L-1}x_s
\end{align*}

\begin{align*}
    \mathcal{L} & = \mathop{\bbE}\limits_{\bX\sim\bbN(0,1)^L}\Bigg[\alpha^2 x_{L-2}^2 +\left(\frac{1}{L-2}\right)^2\sum_{s=2}^{L-1}\exp(2w^*x_Lx_{s-1})x_s^2
    \\& \quad\quad\quad\quad\quad\quad +\frac{\alpha^2}{(L-2)^2}\sum_{\tau=1}^{L-2}\left(\sum_{s=\tau+1}^{L-1}\sm_s(-\tilde{p}(s-1-\tau))\right)^2 x_{\tau}^2+\left(\frac{1}{L-2}\right)^2\sum_{s=2}^{L-1}x_s^2 
    \\& \quad\quad\quad\quad\quad\quad +\frac{2\alpha}{L-2}\exp(w^*x_Lx_{L-3})x_{L-2}^2
    \\& \quad\quad\quad\quad\quad\quad -\frac{2\alpha^2}{L-2}\sm_{L-1}(0)x_{L-2}^2-\frac{2\alpha}{L-2}x_{L-2}^2
    \\& \quad\quad\quad\quad\quad\quad -\frac{2\alpha}{(L-2)^2}\sum_{\tau=2}^{L-2}\left(\sum_{s=\tau+1}^{L-1}\sm_s(-\tilde{p}(s-1-\tau))\right)\exp(w^*x_Lx_{\tau-1})x_{\tau}^2
    \\& \quad\quad\quad\quad\quad\quad -2\left(\frac{1}{L-2}\right)^2\sum_{s=2}^{L-1}\exp(w^*x_Lx_{s-1})x_s^2
    \\& \quad\quad\quad\quad\quad\quad +\frac{2\alpha}{(L-2)^2}\sum_{\tau=1}^{L-2}\left(\sum_{s=\tau+1}^{L-1}\sm_s(-\tilde{p}(s-1-\tau))\right)x_{\tau}^2 \Bigg] 
    \\& = \frac{\alpha^2}{(L-2)^2}\sum_{\tau=1}^{L-2}\left(\sum_{s=\tau+1}^{L-1}\sm_s(-\tilde{p}(s-1-\tau))\right)^2-\frac{2\alpha^2}{L-2}\sm_{L-1}(0)
    \\& \quad + C(p,w,w^*)
\end{align*}

\begin{align*}
    h(\tilde{p}) & := \sum_{\tau=1}^{L-2}\left(\sum_{s=\tau+1}^{L-1}\frac{e^{\tilde{p}(s-1-\tau)}}{\sum_{k=0}^{s-2}e^{-\tilde{p}k}}\right)^2
    \\& = \sum_{\tau=1}^{L-2}\left(\sum_{s=\tau+1}^{L-1}\frac{e^{-\tilde{p}(s-1-\tau)}}{1-e^{-\tilde{p}(s-1)}}(1-e^{-\tilde{p}})\right)^2
    \\& = (1-e^{-\tilde{p}})^2\sum_{\tau=1}^{L-2}\left(\sum_{s=\tau+1}^{L-1}\frac{e^{-\tilde{p}(s-1-\tau)}}{1-e^{-\tilde{p}(s-1)}}\right)^2
    \\& = (1-e^{-\tilde{p}})^2\sum_{\tau=1}^{L-2}e^{2\tilde{p}\tau}\left(\sum_{s=\tau+1}^{L-1}\frac{e^{-\tilde{p}(s-1)}}{1-e^{-\tilde{p}(s-1)}}\right)^2
    \\& = (1-e^{-\tilde{p}})^2\sum_{\tau=1}^{L-2}e^{2\tilde{p}\tau}\left(\sum_{s=\tau+1}^{L-1}\frac{1}{e^{\tilde{p}(s-1)}-1}\right)^2
\end{align*}

\begin{align*}
    h'(\tilde{p}) & = 2(1-e^{-\tilde{p}})e^{-\tilde{p}}\sum_{\tau=1}^{L-2}e^{2\tilde{p}\tau}\left(\sum_{s=\tau+1}^{L-1}\frac{1}{e^{\tilde{p}(s-1)}-1}\right)^2
    \\& + (1-e^{-\tilde{p}})^2\sum_{\tau=1}^{L-2}2\tau e^{2\tilde{p}\tau}\left(\sum_{s=\tau+1}^{L-1}\frac{1}{e^{\tilde{p}(s-1)}-1}\right)^2
    \\& + (1-e^{-\tilde{p}})^2\sum_{\tau=1}^{L-2}2e^{2\tilde{p}\tau}\left(\sum_{s=\tau+1}^{L-1}\frac{1}{e^{\tilde{p}(s-1)}-1}\right)\left(\sum_{s=\tau+1}^{L-1}\frac{-(s-1)e^{\tilde{p}(s-1)}}{(e^{\tilde{p}(s-1)}-1)^2}\right)
    \\& = 2(1-e^{-\tilde{p}})\sum_{\tau=1}^{L-2}e^{2\tilde{p}\tau}\left(\sum_{s=\tau+1}^{L-1}\frac{1}{e^{\tilde{p}(s-1)}-1}\right)\left(\sum_{s=\tau+1}^{L-1}\frac{e^{-\tilde{p}}+\tau(1-e^{-\tilde{p}})}{e^{\tilde{p}(s-1)}-1}-\frac{(s-1)e^{\tilde{p}(s-1)}}{(e^{\tilde{p}(s-1)}-1)^2}\right)
\end{align*}

The numerator of $h'(\tilde{p})$'s last factor is 

\begin{align*}
    & \left(\tau-(\tau-1)e^{-\tilde{p}}\right)\left(e^{\tilde{p}(s-1)}-1\right)-(s-1)e^{\tilde{p}(s-1)}
    \\ =& (\tau+1-s)t^{s-1}-(\tau-1)t^{s-2}-\tau+\frac{\tau-1}{t} 
\end{align*}

where $t=e^{-\tilde{p}}\geq 1$. Since $s\geq \tau+1$, $h'(\tilde{p})\leq 0$.

\begin{align*}
    \frac{d\tilde{p}}{dt} &= -\frac{\alpha^2}{(L-2)^2}h'(\tilde{p})+\frac{2\alpha^2}{L-2}\frac{m(\tilde{p})}{M(\tilde{p})}^2
    \\& \geq \frac{2\alpha^2}{L-2}\frac{m(\tilde{p})}{M(\tilde{p})^2}
\end{align*}

According to the calculation in stage I, $\tilde{p}$ grows like $\ln$.
